# Supplementary material for: Grounded Question-Answering in Long Egocentric Videos
Source: arXiv:2312.06505 source file (2024-04-01)
Supplement: Supplementary file 1 [file supp_closeqa.pdf]

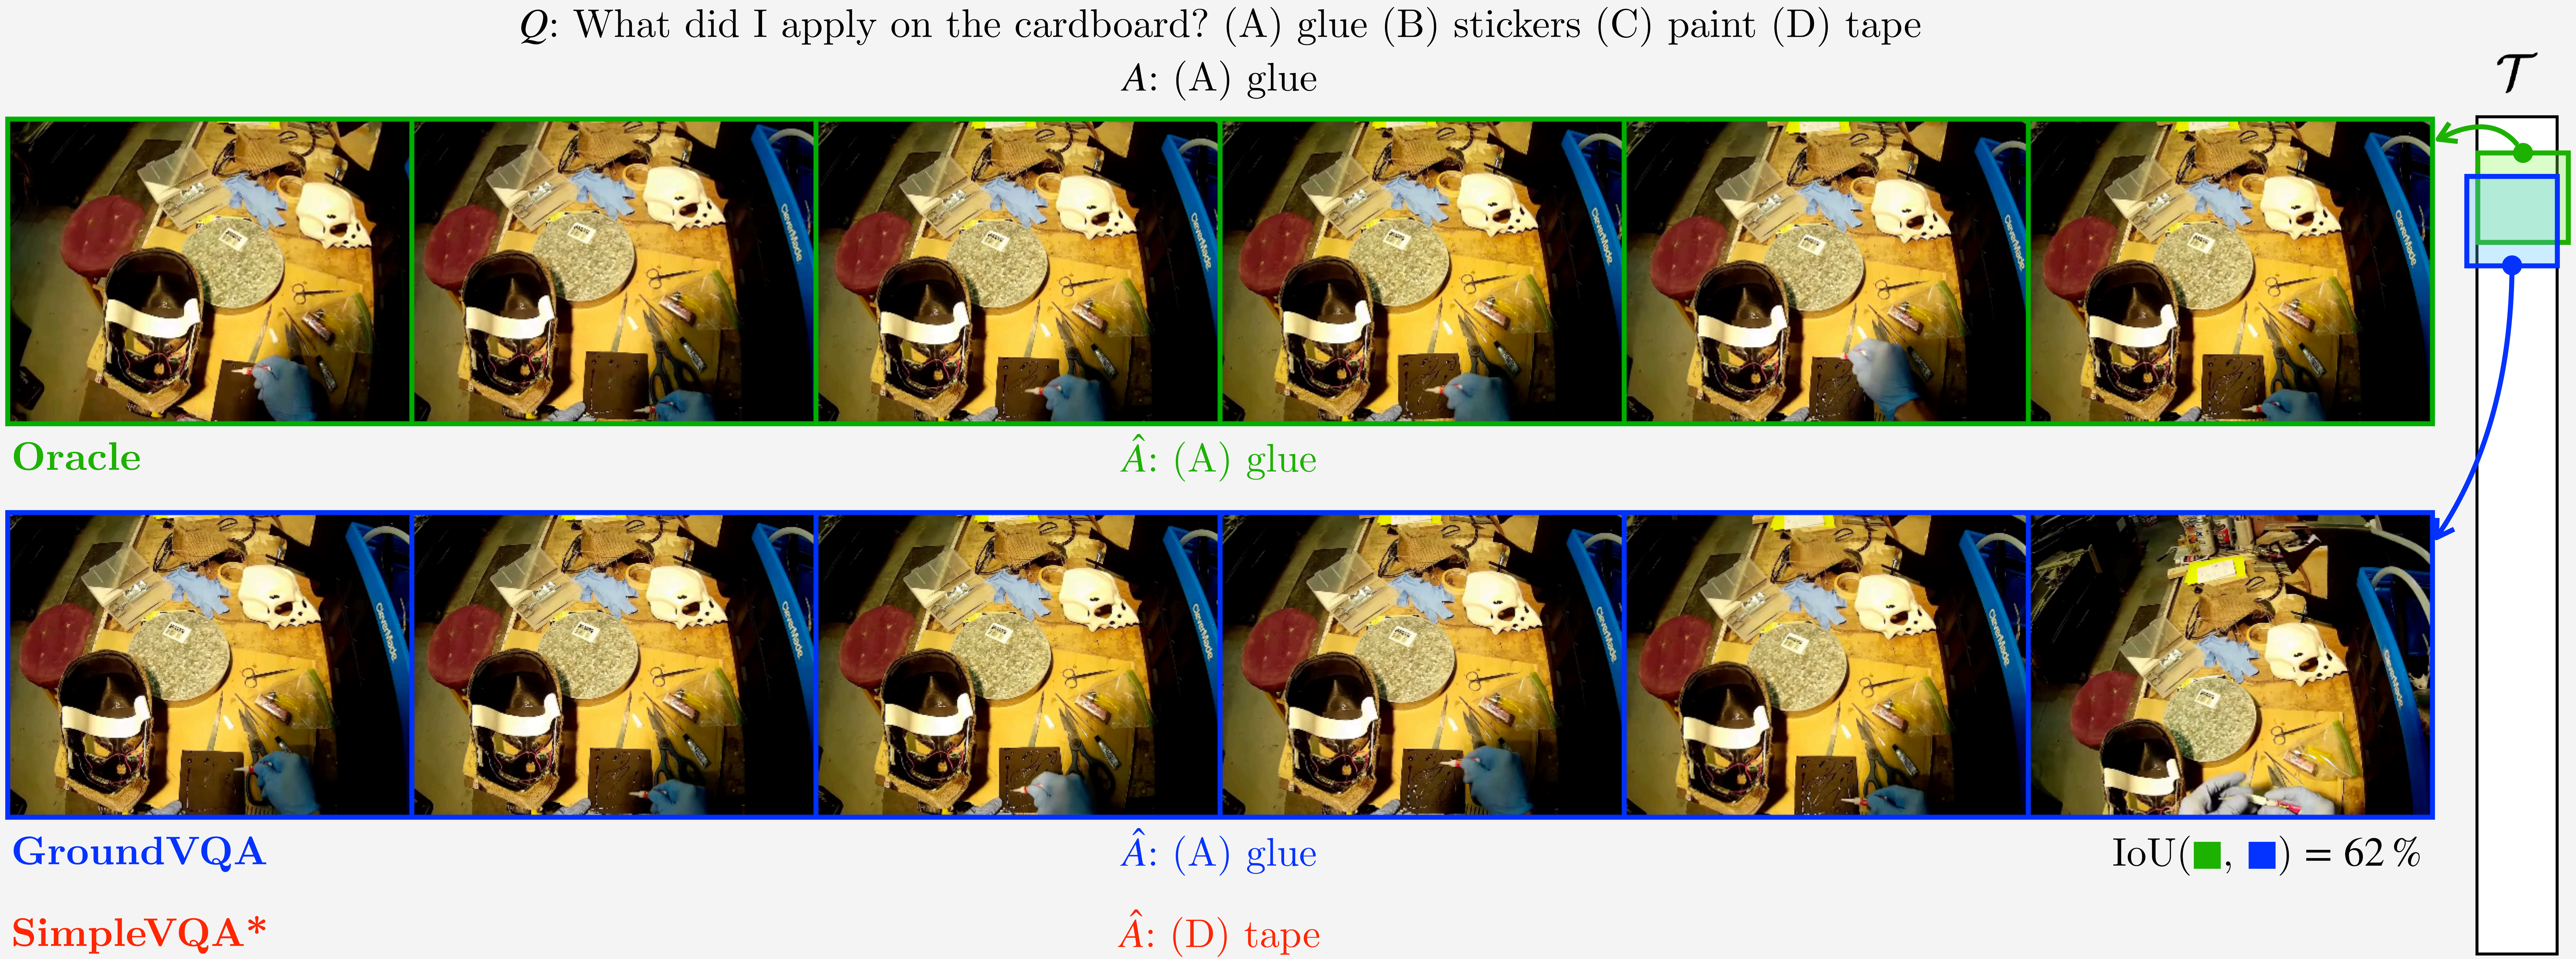
$Q$: What did I apply on the cardboard? (A) glue (B) stickers (C) paint (D) tape
$A$: (A) glue
$\mathcal{T}$
Oracle
$\hat{A}$: (A) glue
GroundVQA
$\hat{A}$: (A) glue
IoU(■, ■) = 62 %
SimpleVQA*
$\hat{A}$: (D) tape

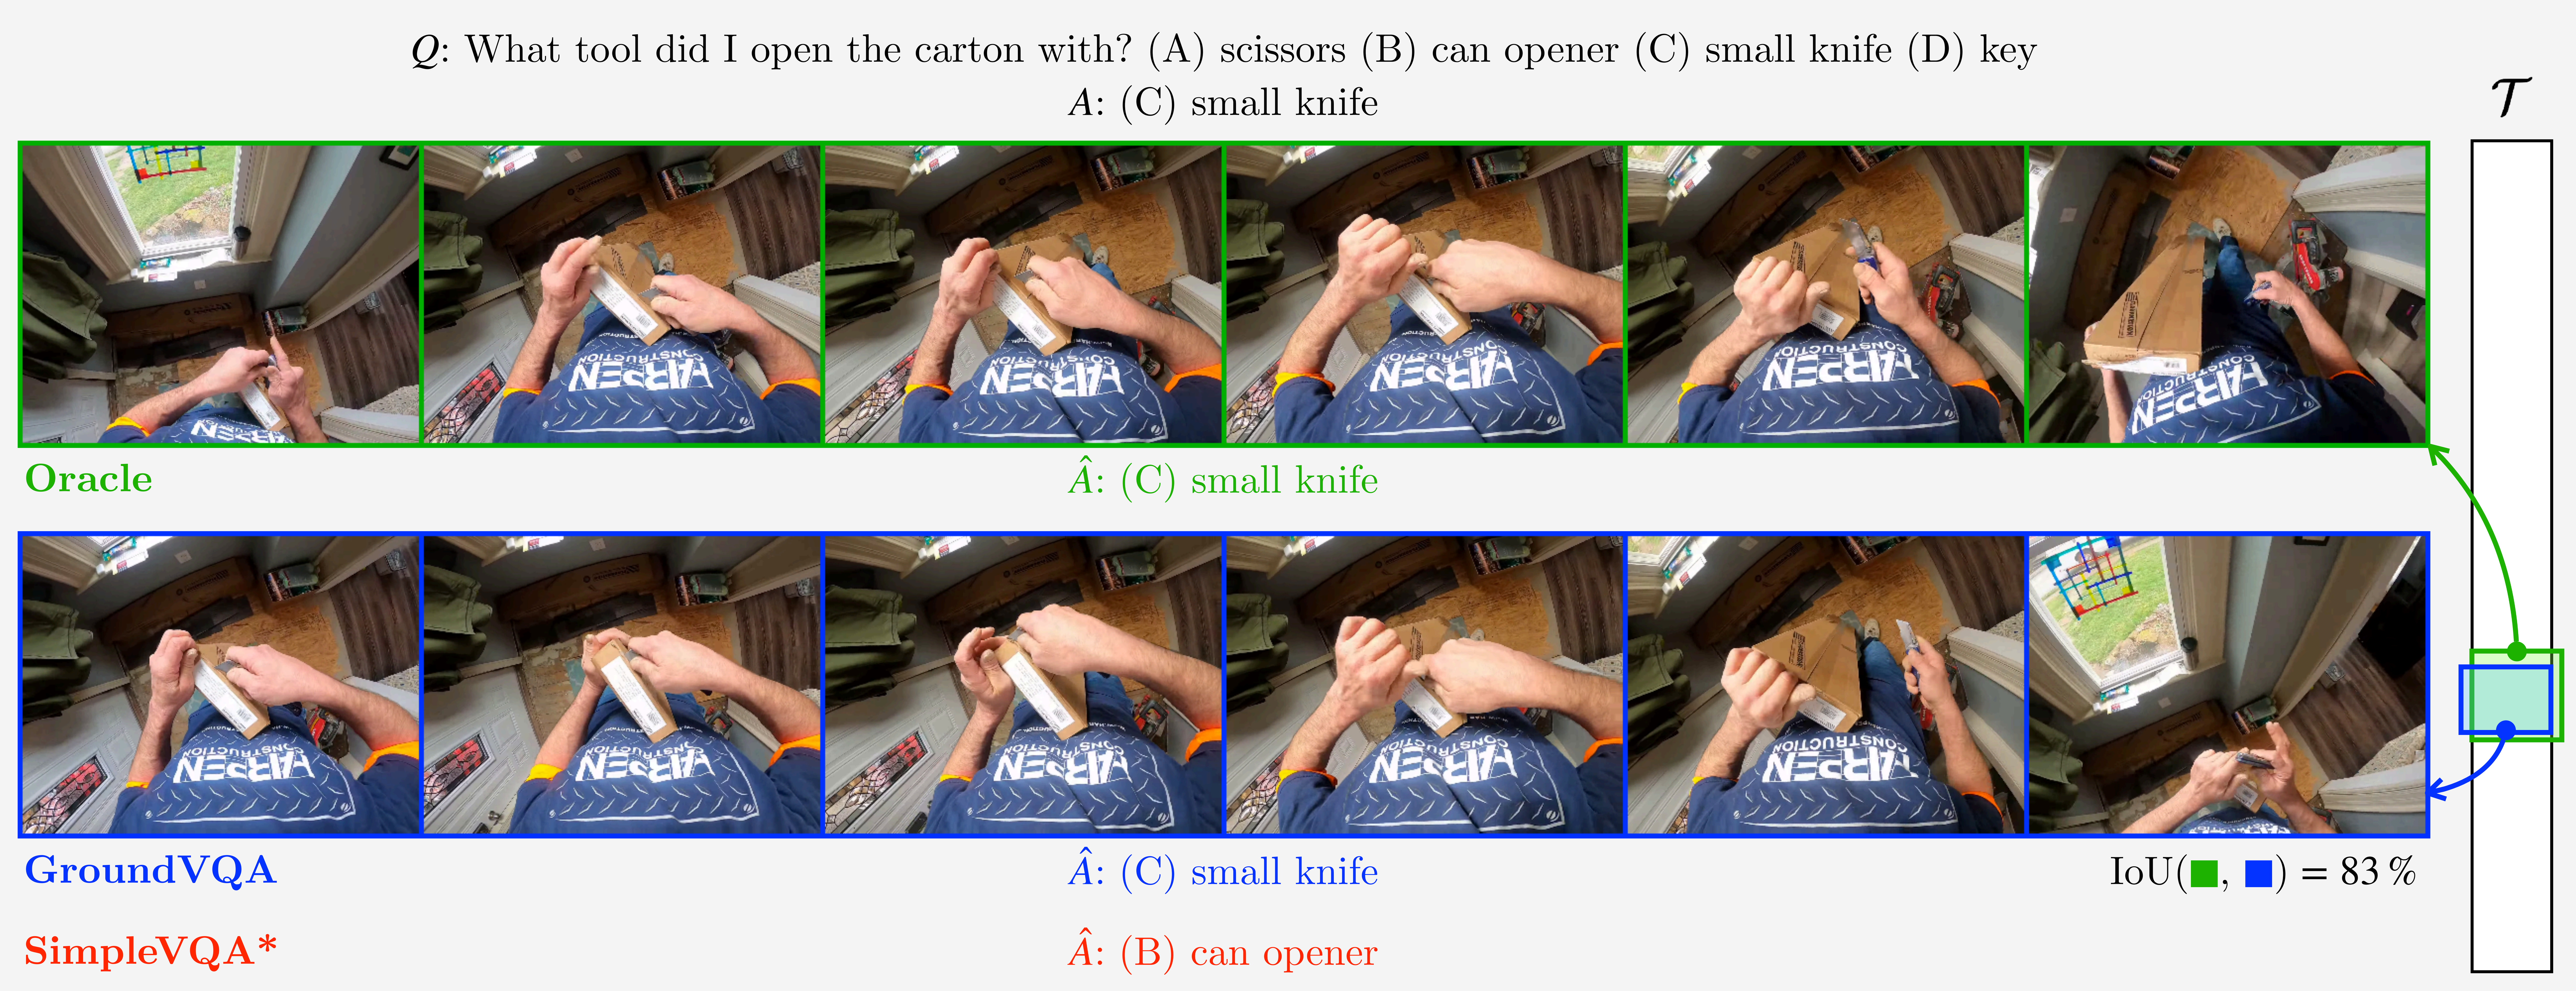
$Q$: What tool did I open the carton with? (A) scissors (B) can opener (C) small knife (D) key
$A$: (C) small knife
$\mathcal{T}$
Oracle
$\hat{A}$: (C) small knife
GroundVQA
$\hat{A}$: (C) small knife
IoU(■, ■) = 83 %
SimpleVQA*
$\hat{A}$: (B) can opener

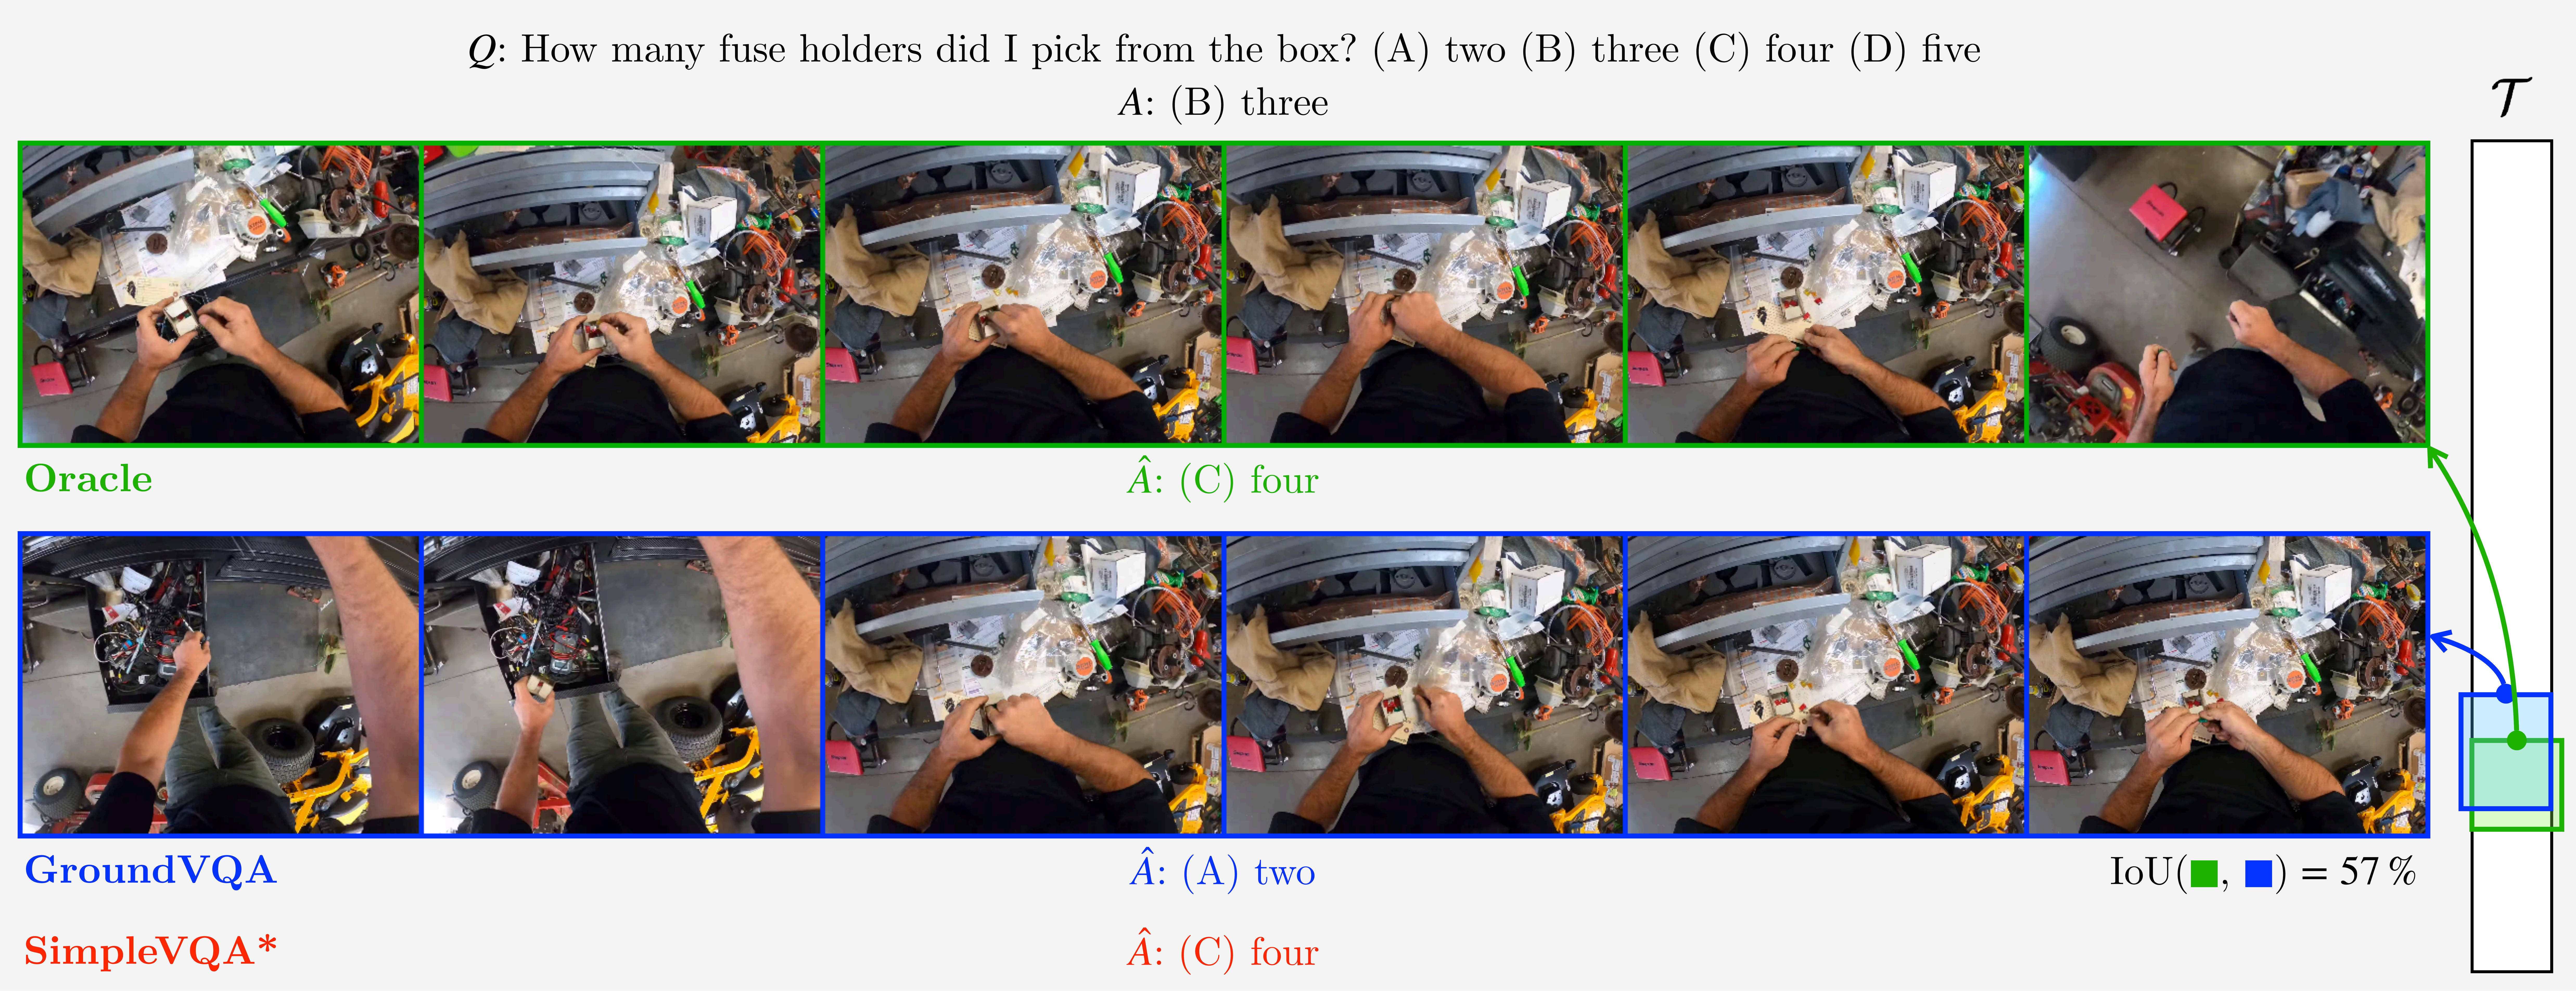

Q: How many fuse holders did I pick from the box? (A) two (B) three (C) four (D) five
A: (B) three
𝒯
Oracle
Â: (C) four
GroundVQA
Â: (A) two
IoU(■, ■) = 57 %
SimpleVQA*
Â: (C) four

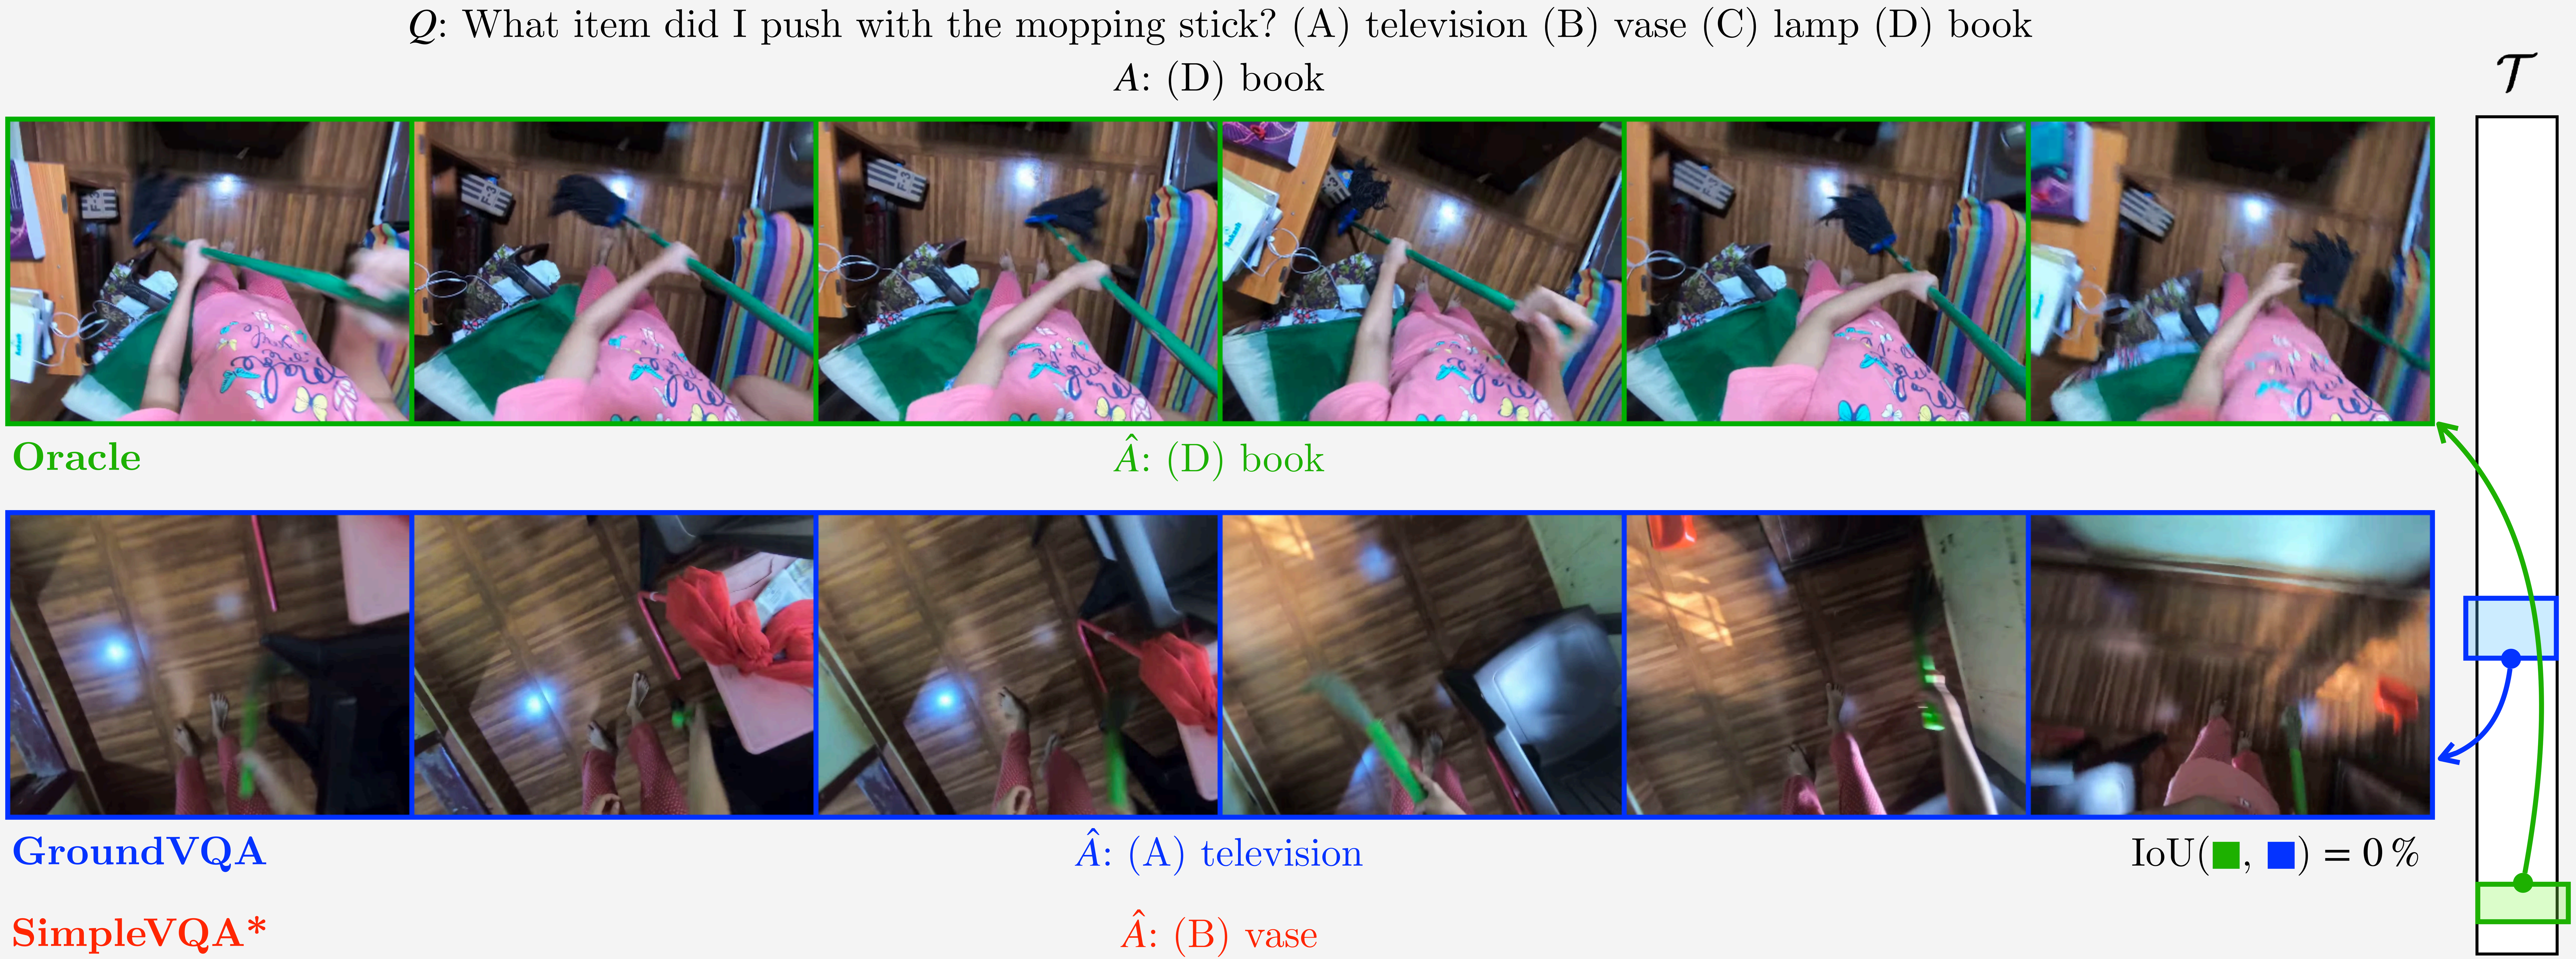
$Q$: What item did I push with the mopping stick? (A) television (B) vase (C) lamp (D) book
$A$: (D) book
$\mathcal{T}$
Oracle
$\hat{A}$: (D) book
GroundVQA
$\hat{A}$: (A) television
IoU(■, ■) = 0 %
SimpleVQA*
$\hat{A}$: (B) vase
