# Supplementary material for: Grounded Question-Answering in Long Egocentric Videos
Source: arXiv:2312.06505 source file (2024-04-01)
Supplement: Supplementary file 2 [file supp_openqa.pdf]

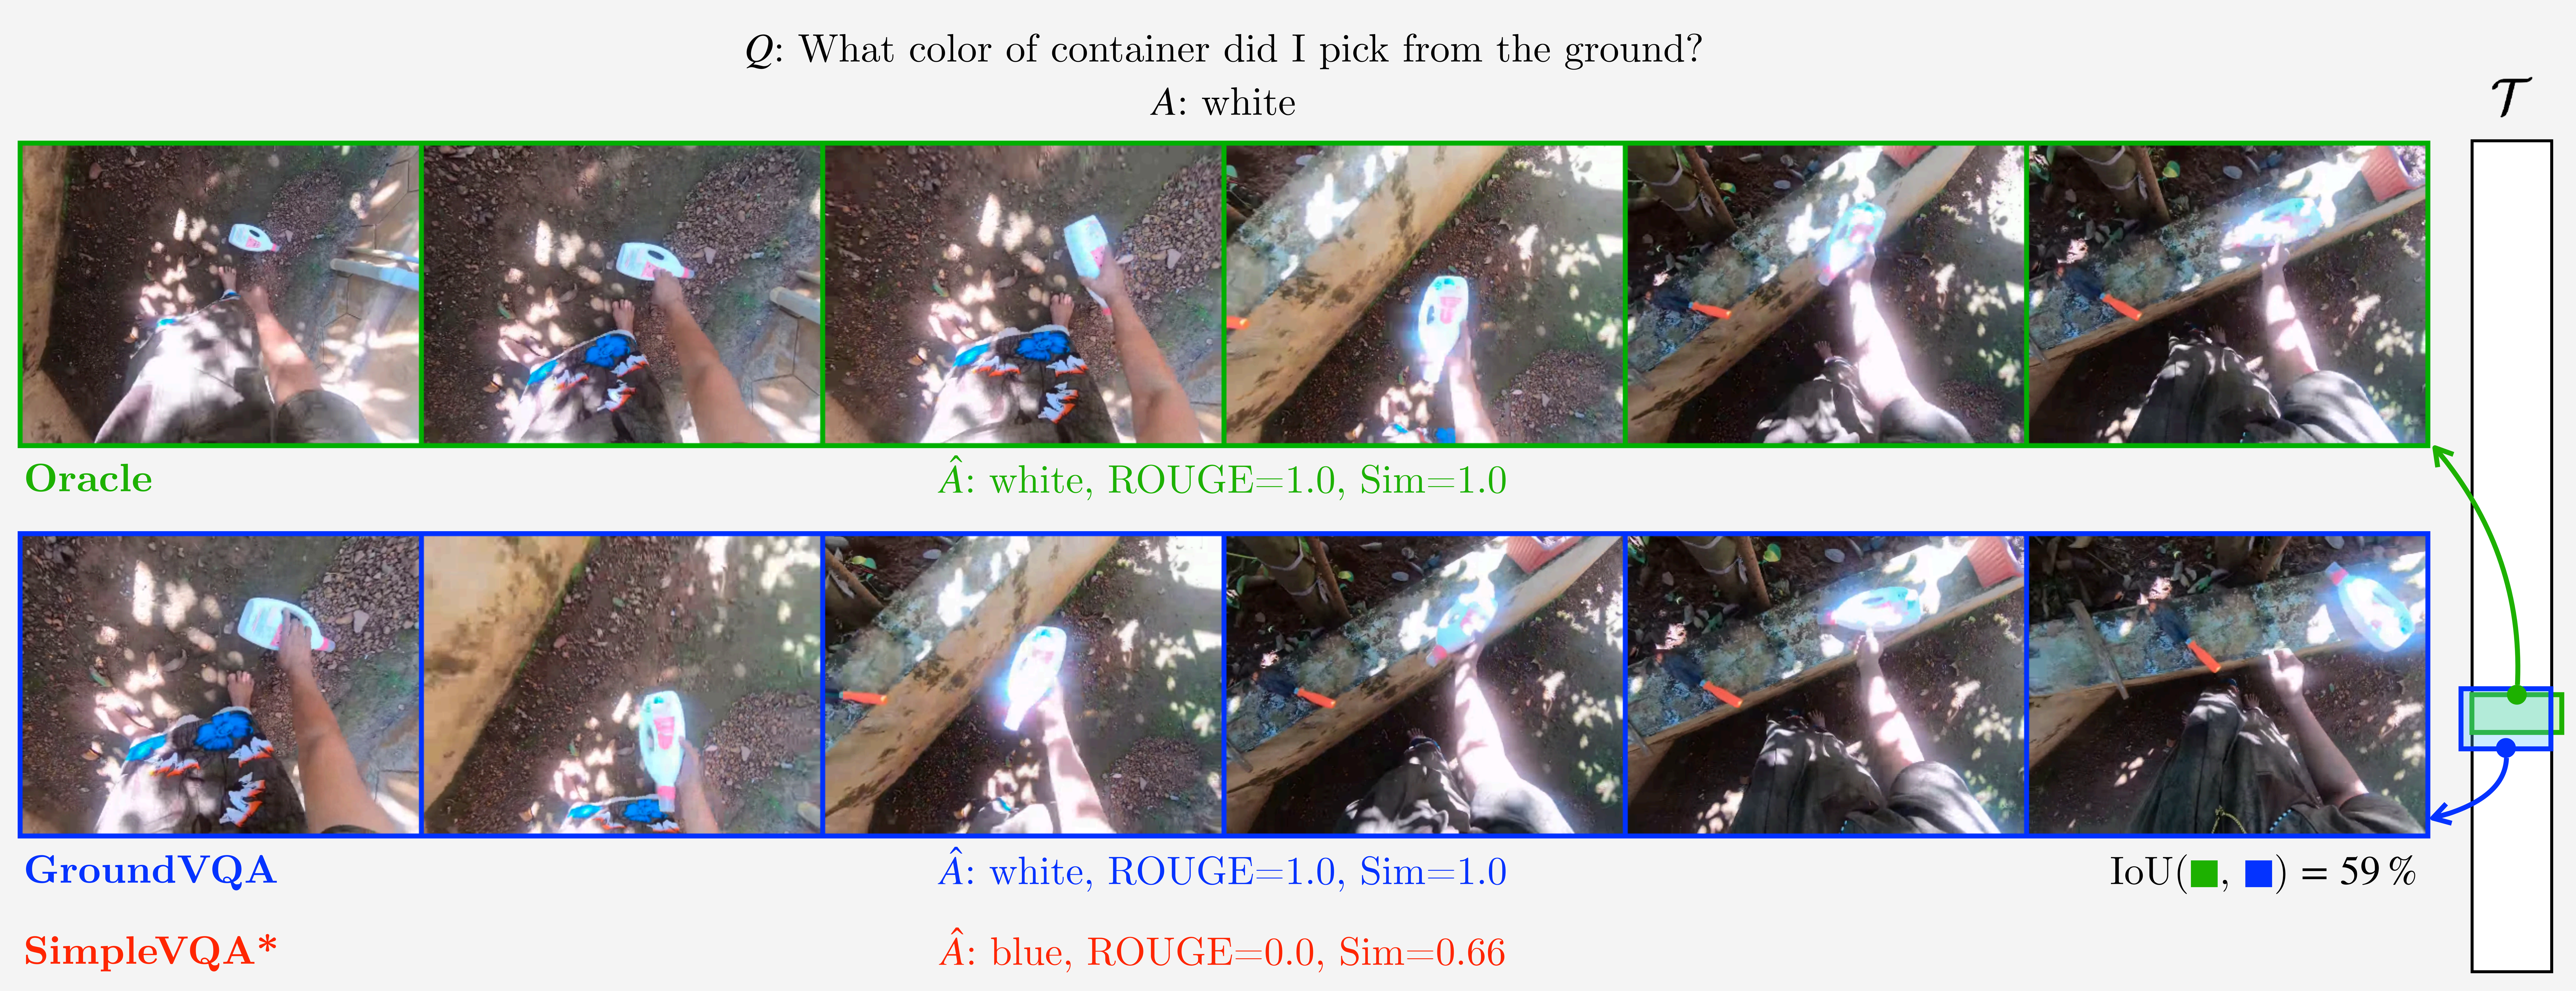

Q: What color of container did I pick from the ground?
A: white
𝒯
Oracle
Â: white, ROUGE=1.0, Sim=1.0
GroundVQA
Â: white, ROUGE=1.0, Sim=1.0
IoU(■, ■) = 59 %
SimpleVQA*
Â: blue, ROUGE=0.0, Sim=0.66

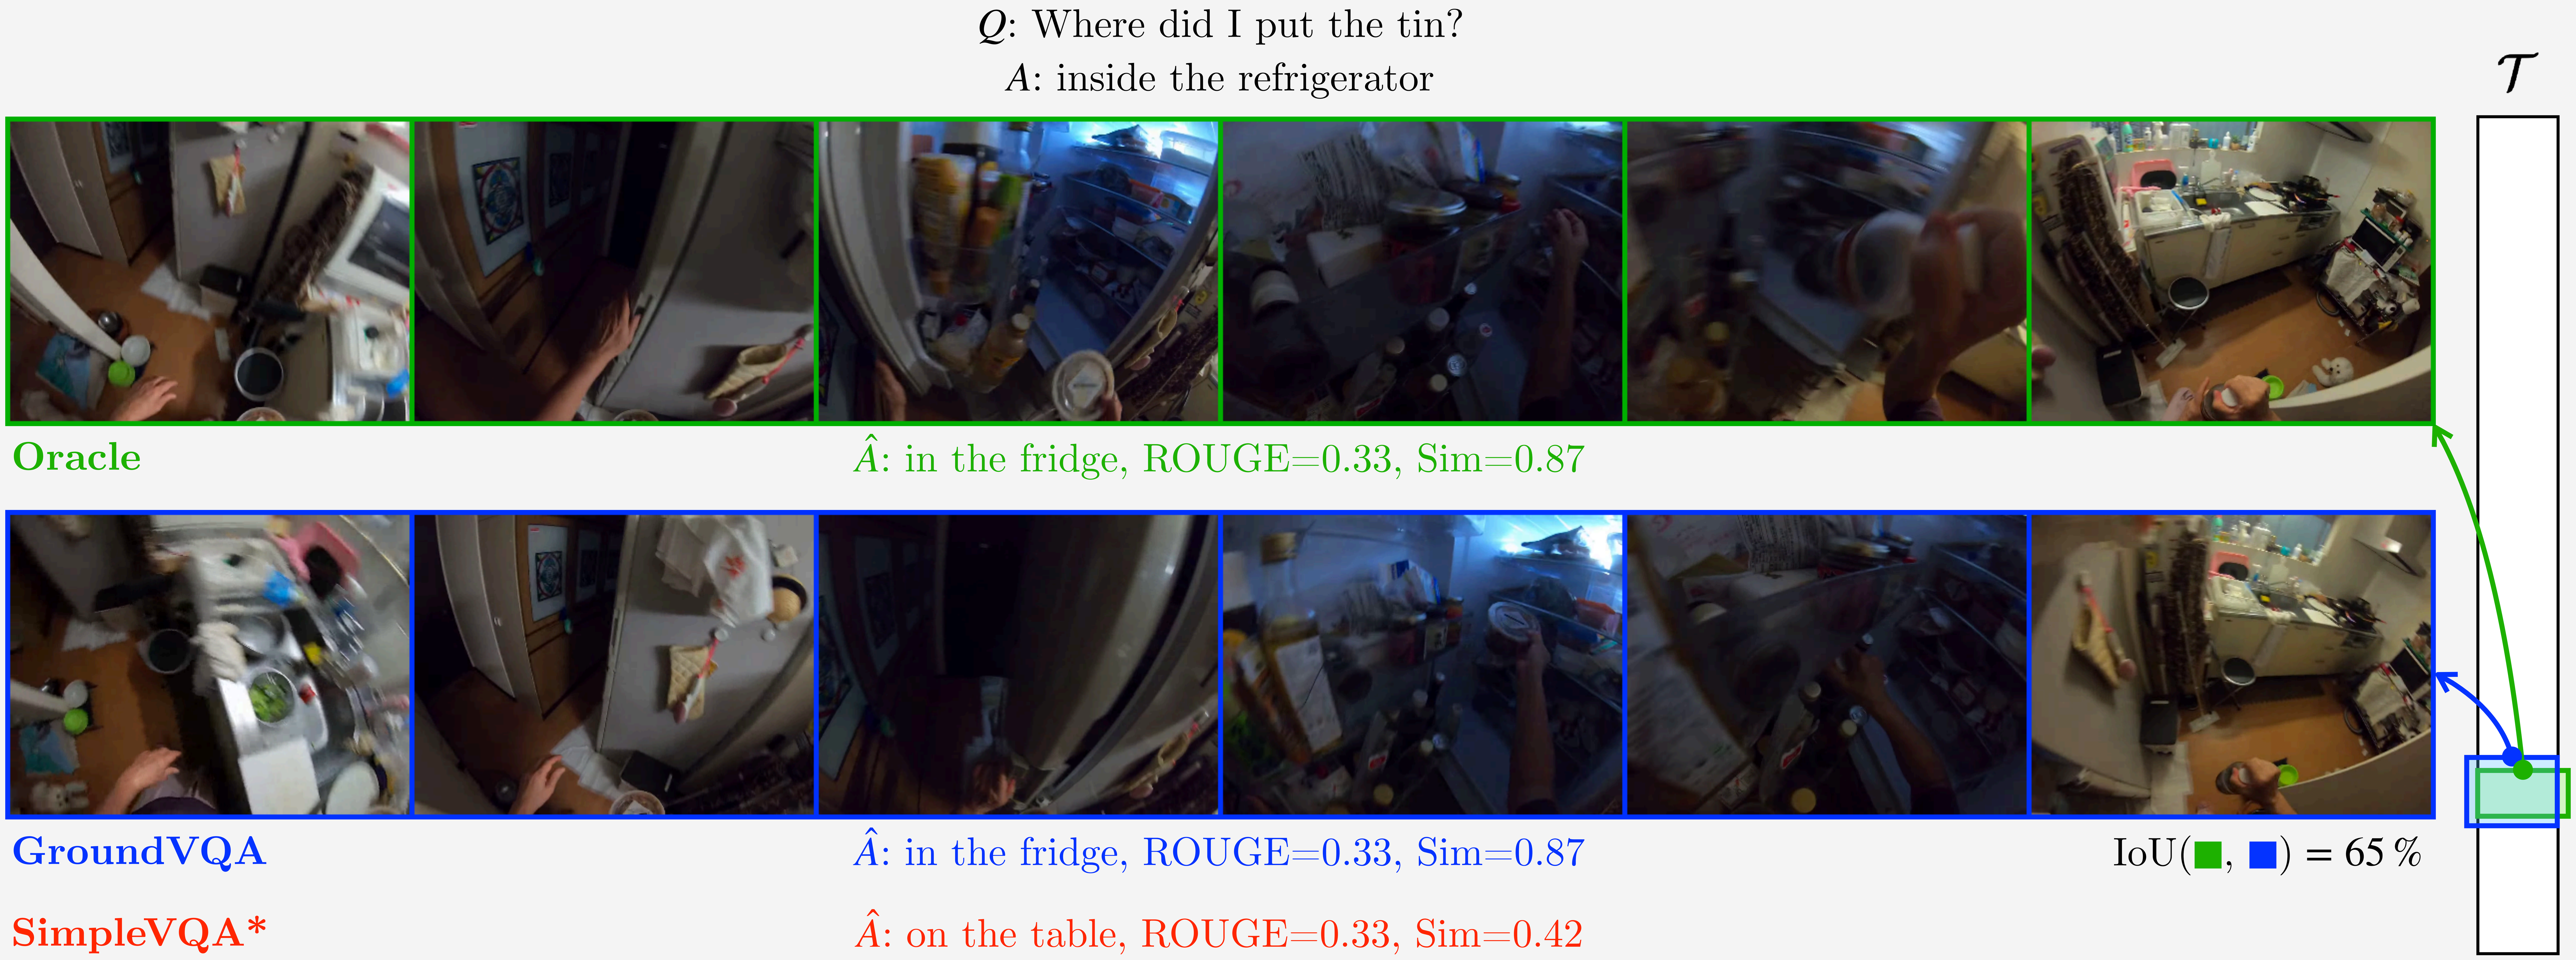

Q: Where did I put the tin?
A: inside the refrigerator
Oracle
Â: in the fridge, ROUGE=0.33, Sim=0.87
GroundVQA
Â: in the fridge, ROUGE=0.33, Sim=0.87
IoU(■, ■) = 65 %
SimpleVQA*
Â: on the table, ROUGE=0.33, Sim=0.42
𝒯

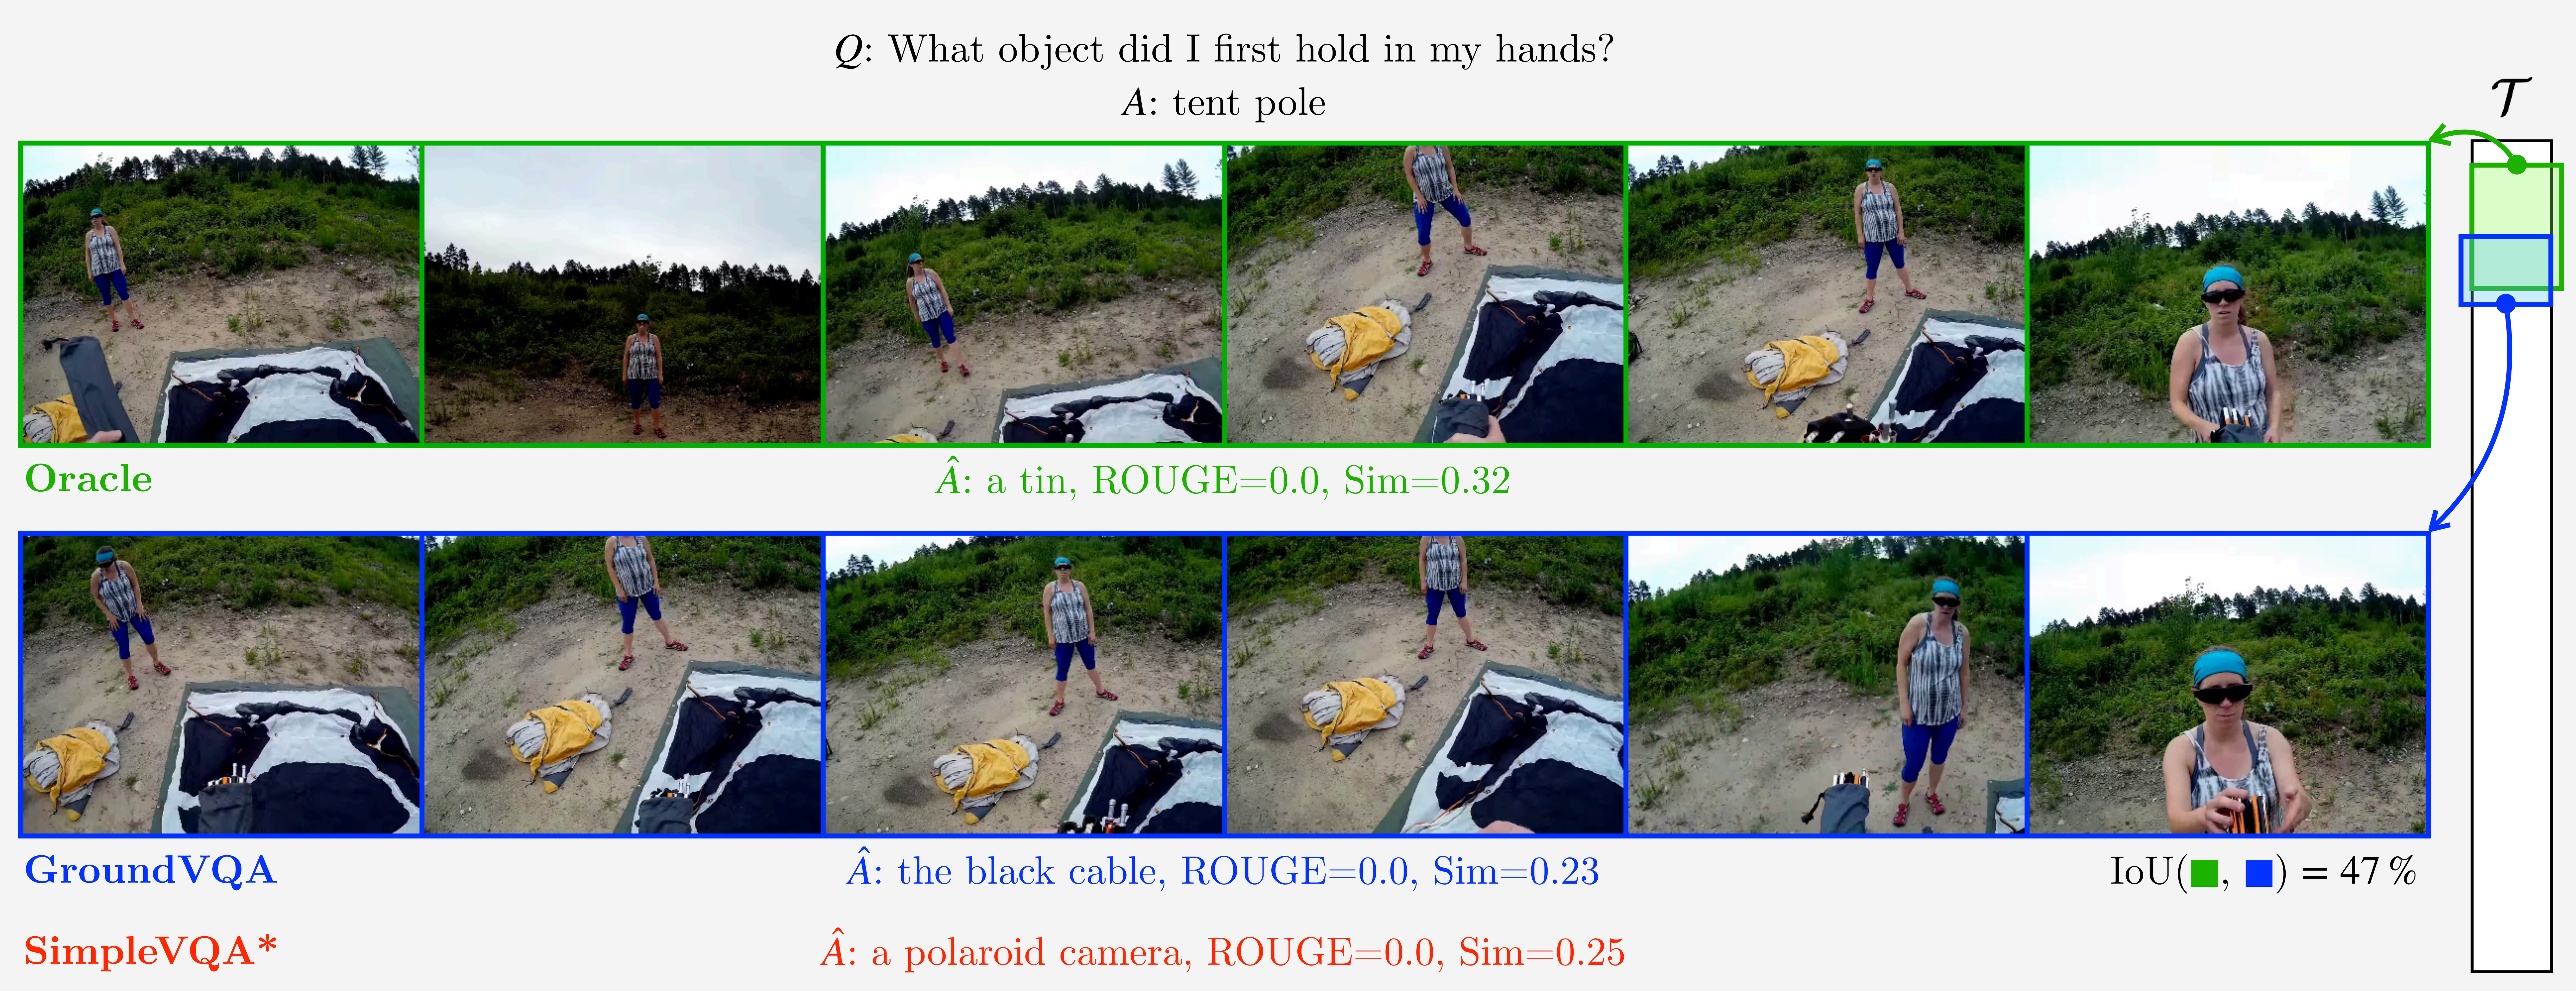
Q: What object did I first hold in my hands?
A: tent pole
Oracle
Â: a tin, ROUGE=0.0, Sim=0.32
GroundVQA
Â: the black cable, ROUGE=0.0, Sim=0.23
IoU( , ) = 47 %
SimpleVQA*
Â: a polaroid camera, ROUGE=0.0, Sim=0.25
𝒯

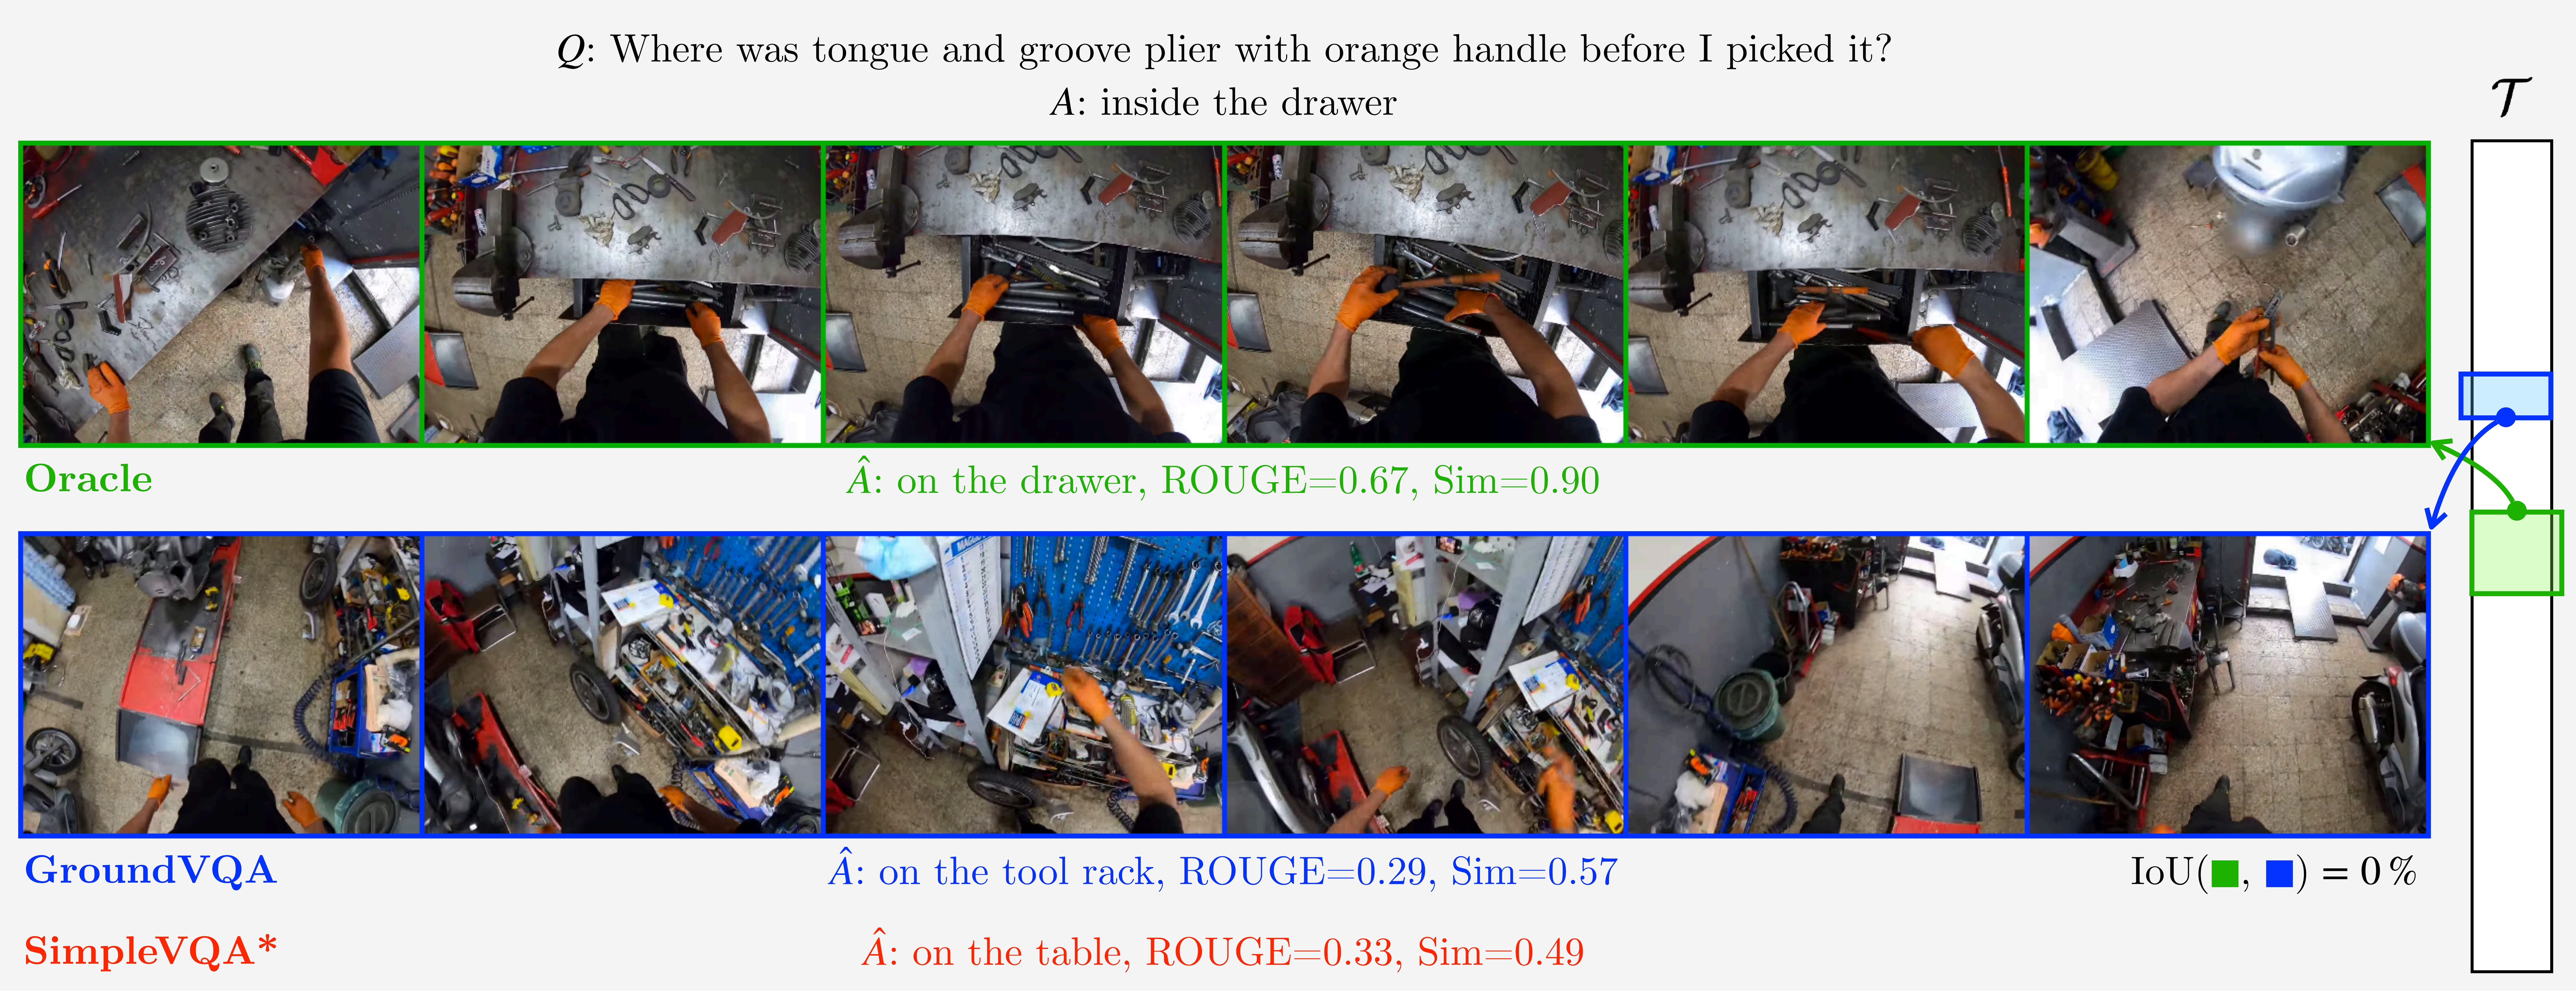

$Q$: Where was tongue and groove plier with orange handle before I picked it?
$A$: inside the drawer
$\mathcal{T}$
Oracle
$\hat{A}$: on the drawer, ROUGE=0.67, Sim=0.90
GroundVQA
$\hat{A}$: on the tool rack, ROUGE=0.29, Sim=0.57
IoU(■, ■) = 0 %
SimpleVQA*
$\hat{A}$: on the table, ROUGE=0.33, Sim=0.49
